# Supplementary material for: Large-Scale QA-SRL Parsing
Source: arXiv:1805.05377 source file (2018-05-14)
Supplement: Supplementary file 1 [file supplementary.tex]

\appendix

\section{Supplemental Material}
\label{sec:supplemental}

\subsection{Experimental Setup}

\paragraph{Hyperparameters}

The parameters of our LSTMs are initialized with random orthonormal matrices as described
by~\newcite{saxe2013exact}.
Input tokens are lower-cased, and the word vectors are pre-initialized with the 100-dimensional
Glove embeddings trained on 6B tokens~\citep{pennington2014glove} and fine-tuned during training.
Tokens which are not covered by the Glove embeddings are assigned to the UNK vector. The embedding
of the binary predicate indicator feature is also 100 dimensions.
The text-encoder BiLSTM consists of 4 layers, uses a hidden size of 300 and .
The output prediction feed-forward neural network for each model consists of a single 100 dimensional
hidden layer with the non-rectified linear unit nonlinearity.
For the sequential question generation model, each timestep consists of 4 layers of LSTMCells with a hidden
size of 200.

\paragraph{Training}

All models are trained using Adadelta~\citep{zeiler2012adadelta} with $\epsilon=1e^{-6}$ and $\rho = 0.95$ and a mini-batch size of 80.
The span encoding BiLSTM uses a recurrent dropout rate of 0.1, and we clip gradients with a norm greater than 1.
All models were trained until performance on the development set did not improve for 10 epochs\footnote{All models
completed training within 40 epochs, which took less than 4 hours on a single Titan X Pascal GPU.}.
Our models were implemented in PyTorch\footnote{\url{http://pytorch.org/}} using the AllenNLP toolkit~\citep{gardnerallennlp}.
